# Supplementary material for: Sharpness-diversity tradeoff: improving flat ensembles with SharpBalance
Source: arXiv:2407.12996 source file (2024-07-17)
Supplement: Supplementary file 1 [file appendix_corr.tex]

\section{Corroborating results on ensembling improvement}
\label{abl:corr-res}

\begin{figure}[!th]
\centering
\begin{subfigure}{0.30\linewidth}
\includegraphics[width=\linewidth,keepaspectratio]{figs/trade_off/dense_cifar10_trade_off_corr_der_EIR.pdf} 
\caption{\footnotesize CIFAR-10}  % (S=0)
\end{subfigure}  
\begin{subfigure}{0.30\linewidth}
\includegraphics[width=\linewidth,keepaspectratio]{figs/trade_off/dense_resnet18_cifar100_trade_off_corr_worst_ltwo0.5_der_EIR.pdf} 
\caption{\footnotesize CIFAR100}  % (S=0)
\centering
\end{subfigure}
\begin{subfigure}{0.30\linewidth}
\includegraphics[width=\linewidth,keepaspectratio]{figs/trade_off/dense_resnet18_10_tin_trade_off_corr_worst_ltwo0.5_der_EIR.pdf} 
\caption{\footnotesize TIN} 
\end{subfigure}  
\centering
\caption{
\textbf{(Sharpness-diversity tradeoff hurts ensemble improvement over single model}). 
Decreasing the sharpness of individual models leads to a lower ensemble improvement ratio (EIR) due to decreased diversity. 
}\label{fig:tradeoff-data-arch-EIR}
\end{figure}

This section shows the results of evaluating the effectiveness of ensembling in the sharpness-diversity trade-off. 
This is measured by the metric called ensemble improvement ratio (EIR)~\cite{theisen2023ensembles}, which is defined as the ensembling improvement over the average performance of single models.
Let $\mathcal{E}_\text{ens}$ denote the test error of an ensemble; 
the EIR is then defined as follows:
\begin{equation}\label{eqn:eir}
\text{EIR}=\frac{ E_{\theta \sim P}[\mathcal{E}(f_\theta)] - \mathcal{E}_\text{ens} }{ E_{\theta \sim P}[\mathcal{E}(f_\theta)] }.
\end{equation}

Note that all the notations here are detailed in the main paper Section~\ref{sec:notation}.
The experimental setup is detailed in Section~\ref{sec:flat-div}.
From Figure~\ref{fig:tradeoff-data-arch-EIR}, 
We indeed observe that, from right to left, when the sharpness decreases and the diversity decreases, the EIR (color of the marker changes from red to blue) also decreases.
It demonstrates that ensembling becomes less beneficial compared to individual NN, and the sharpness-diversity trade-off has an adverse effect on the overall ensembling performance.
